# Supplementary material for: Observation of Phase Controllable Majorana-like Bound States in Metamaterial-based Kitaev Chain Analogues
Source: arXiv:2201.12377 ancillary file (2022-01-28)
Supplement: Supplementary file 1 [file Supp-Mat.pdf]

# Supplemental Material for "Observation of Phase Controllable Majorana-like Bound States in Metamaterial-based Kitaev Chain Analogues"

Kai Qian,[1] David J. Apigo,[1] Karmela Padavić,[2] Keun Hyuk Ahn,[1] Smitha Vishveshwara,[2] and Camelia Prodan[1]

[1]*Department of Physics, New Jersey Institute of Technology, Newark, New Jersey, 07102, USA*

[2]*Department of Physics, University of Illinois at Urbana-Champaign, Urbana, Illinois, 61801, USA*

## I. DETAILS OF EXPERIMENTAL SETUP

The system is made of two parallel SSH chains with alternating *intrachain* couplings, shifted with respect to each other and coupled by a constant *interchain* interaction. Each spinner has six arms with magnets attached to the arms in the 0°, 180°, and 240° [0°, 60° and 180°] directions for the top [bottom] chain, as highlighted in Fig. 1(a) in the main text. The red, blue, and green lines in Fig. 1(b) indicate different nearest-neighbor interactions, represented by the normalized positive parameters, $\beta_r$, $\beta_b$, and $\beta_g$ between the magnets separated by the distances, $d_r$=5.0 mm, $d_b$=8.0 mm, and $d_g$, respectively. The root mean square voltages from attached accelerometers divided by frequency squared ($f^2$) are used as the quantities proportional to the oscillation amplitudes. Further details of the setup are provided in Refs. [S1, S2, S3].

## II. TYPICAL SPECTRA, GAP VERSUS INTERCHAIN COUPLING $\beta_g$, AND THEORETICAL RANGES FOR BULK BANDS

Typical spectra of the normalized amplitude versus $f^2$ for the long $N$=13 ladder systems are shown in Figs. S1(a), S1(b), and S1(c) for the topological insulator, metallic, and nontopological insulator cases, respectively (see the left panels in Fig. 1 in the main text).

According to the theory [S4] for the infinitely long SSH ladder system, the outer boundaries of the bulk bands are at

$$f^2 = \alpha \pm (\beta_r + \beta_b + \beta_g), \tag{1}$$

while the inner boundaries are at

$$f^2 = \alpha \pm |\beta_r + \beta_b - \beta_g|, \text{ if } \beta_g > \beta_{g,G}, \tag{2}$$

$$f^2 = \alpha \pm |\beta_r - \beta_b| \sqrt{1 - \beta_g^2/4\beta_b\beta_r}, \text{ if } \beta_g < \beta_{g,G}, \tag{3}$$

where

$$\beta_{g,G} = 4\beta_b\beta_r/(\beta_b + \beta_r). \tag{4}$$

With the parameters for the systems studied, we obtain $\beta_{g,G}$ = 280 Hz$^2$ indicated on the top axis in Fig. S1(d), and the ranges for the upper and lower bulk bands shown as the gray areas in Fig. 1(c) in the main text. The theoretical gap size $G_{\text{theory}}$ is found to be

$$G_{\text{theory}} = 2|\beta_r + \beta_b - \beta_g|, \text{ if } \beta_g > \beta_{g,G}, \tag{5}$$

$$G_{\text{theory}} = 2|\beta_r - \beta_b| \sqrt{1 - \beta_g^2/4\beta_b\beta_r}, \text{ if } \beta_g < \beta_{g,G}. \tag{6}$$

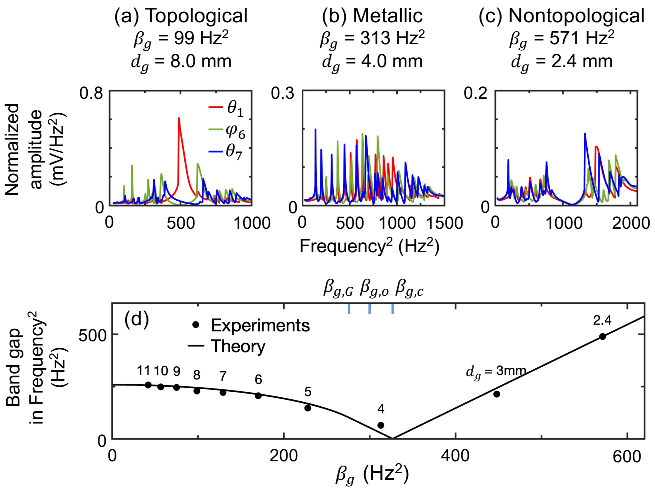


FIG. S1. (a), (b), and (c): Spectra measured for the long $N$=13 ladder systems with the interchain coupling $\beta_g$ = 99, 313, and 571 Hz$^2$ to show the examples of the spectra for the topological insulator, metallic, and nontopological insulator phases, respectively. The red, green, and blue lines represent the spectra obtained by actuating the $\theta_1$, $\varphi_6$, and $\theta_7$ spinners, respectively, and measuring at the same spinners. Each peak corresponds to a mode, shown as a dot in Fig. 1(c) in the main text. The peak for the mid-gap MLBS is prominent in the topological phase, as seen from the red line in (a), and is represented as a red dot in Fig. 1(c). (d) Band gap versus $\beta_g$, showing topological phase transition as $\beta_g$ decreases from around 600 Hz$^2$. The dots and lines represent the experimental and theoretical results, respectively. The numbers above the dots represent the intermagnet distances, $d_g$, between the two SSH chains. The three tick marks on the top axis represent the three critical values of $\beta_g$, that is, $\beta_{g,c}$ for the gap closing, $\beta_{g,o}$ for the oscillatory MLBS spatial profile, and $\beta_{g,G}$ for the gap function, as discussed in the main text and the text here.

The gap sizes versus the interchain coupling $\beta_g$ for the experiments and theory are displayed as dots and lines, respectively, in Fig. S1(d), showing a good agreement.

## III. DETAILS OF MLBS SPATIAL PROFILE FROM THEORY

The theory [S5] predicts that the MLBS localized at the left edge for the infinitely long ladder system satisfies

the following relations:

$$\varphi_n = 0, \tag{7}$$
$$\theta_{n+1} = -\theta_n \beta_g/\beta_r - \theta_{n-1}\beta_b/\beta_r, \tag{8}$$
$$\theta_2 = -\theta_1 \beta_g/\beta_r. \tag{9}$$

Depending on the sign of $\beta_g - \beta_{g,o}$, where

$$\beta_{g,o} = 2\sqrt{\beta_b \beta_r} < \beta_{g,c}, \tag{10}$$

the solution for $\theta_n$ has different forms:

$$\theta_n = Ae^{-n/\xi}\cos(B + 2n\pi/\lambda),\ \text{if}\ \beta_g < \beta_{g,o}, \tag{11}$$
$$\theta_n = (A + Bn)e^{-n/\xi},\ \text{if}\ \beta_g = \beta_{g,o}, \tag{12}$$
$$\theta_n = Ae^{-n/\xi_+} + Be^{-n/\xi_-},\ \text{if}\ \beta_{g,o} < \beta_g < \beta_{g,c}, \tag{13}$$

where

$$\xi = 2[\ln(\beta_r/\beta_b)]^{-1} \tag{14}$$
$$\xi_\pm = 1/\ln\{2\beta_r/[\beta_g \pm ({\beta_g}^2 - 4\beta_b\beta_r)^{1/2}]\} \tag{15}$$

are the localization lengths,

$$\lambda = 2\pi/\arccos(-\beta_g/2\sqrt{\beta_r\beta_b}) \tag{16}$$

is the wavelength, and $A$ and $B$ are constants.

## IV. DESCRIPTIONS OF SUPPLEMENTAL VIDEOS

Following slow motion videos for figures in the main text are also provided as Supplemental Material.

- Fig1g_video.mp4: Lower MLBS for $N$=5 at $f^2$=486 Hz$^2$
- Fig1i_video.mp4: Upper MLBS for $N$=5 at $f^2$=518 Hz$^2$
- Fig2a_video.mp4: Upper bulk mode for $N$=13 at $f^2$=713 Hz$^2$
- Fig2b_video.mp4: Mid-gap MLBS for $N$=13 at $f^2$=511 Hz$^2$
- Fig2c_video.mp4: Lower bulk mode for $N$=13 at $f^2$=204 Hz$^2$


[S1] D. J. Apigo, K. Qian, C. Prodan, and E. Prodan, Topological edge modes by smart patterning, Phys. Rev. Mater. **2**, 124203 (2018).

[S2] K. Qian, D. J. Apigo, C. Prodan, Y. Barlas, and E. Prodan, Topology of the valley-Chern effect, Phys. Rev. B **98**, 155138 (2018).

[S3] K. Qian, L. Zhu, K. H. Ahn, and C. Prodan, Observation of flat frequency bands at open edges and antiphase boundary seams in topological mechanical metamaterials, Phys. Rev. Lett. **125**, 225501 (2020).

[S4] K. Padavić, S. S. Hegde, W. DeGottardi, and S. Vishveshwara, Topological phases, edge modes, and the Hofstadter butterfly in coupled Su-Schrieffer-Heeger systems, Phys. Rev. B **98**, 024205 (2018).

[S5] S. S. Hegde and S. Vishveshwara, Majorana wavefunction oscillations, fermion parity switches, and disorder in Kitaev chains, Phys. Rev. B **94**, 115166 (2016).
